# Supplementary material for: Entropic Score metric: Decoupling Topology and Size in Training-free NAS
Source: arXiv:2310.04179 source file (2023-10-06)
Supplement: Supplementary file 1 [file supplementary_temp.tex]

\section{ESFormer Architectures}

Figure~\ref{fig:nets} shows the detailed architectures of ESFormer model family: S0 (left), S1 (center), S2 (right). 

It is possible to notice how IBN~\cite{mobilenetV2} constitutes the main building block, especially in the first stages. ConvNeXt~\cite{convnext} is instead preferred in the last stages, with stage 4 usually dominated by this kind of block. 

Similarly, another interesting pattern can be seen in the configuration choice for the FNN in Transformer Encoder layers, with Inverted Bottlenecks usually preferred in stage 3 and ConvNeXt blocks in stage 4. 

With regard to kernel sizes, there is a tendency in the adoption of larger kernels as the depth of the network increases, especially in S0 and S1. This is the same arrangement explicitly devised by the authors of EdgeNeXt~\cite{edgenext}, where the kernel size is maintained small in the first stages to capture low-level features and it is gradually increased to deal with more high-level features. 

Finally, we can appreciate how the QKV-dimension is always consistenly lower than the embedding dimension, except for S2 stage 3. Indeed, it is shown that adopting a smaller QKV-dimension enables a decrease in model complexity without affecting the performance~\cite{searching}.

Notably, while these behaviours are manually encoded in state-of-the-art architectures, they spontaneously emerge in our models during the search thanks to Entropic Score.

%
\begin{figure*}[t]
    \centering
        \includegraphics[width=1.9\columnwidth]{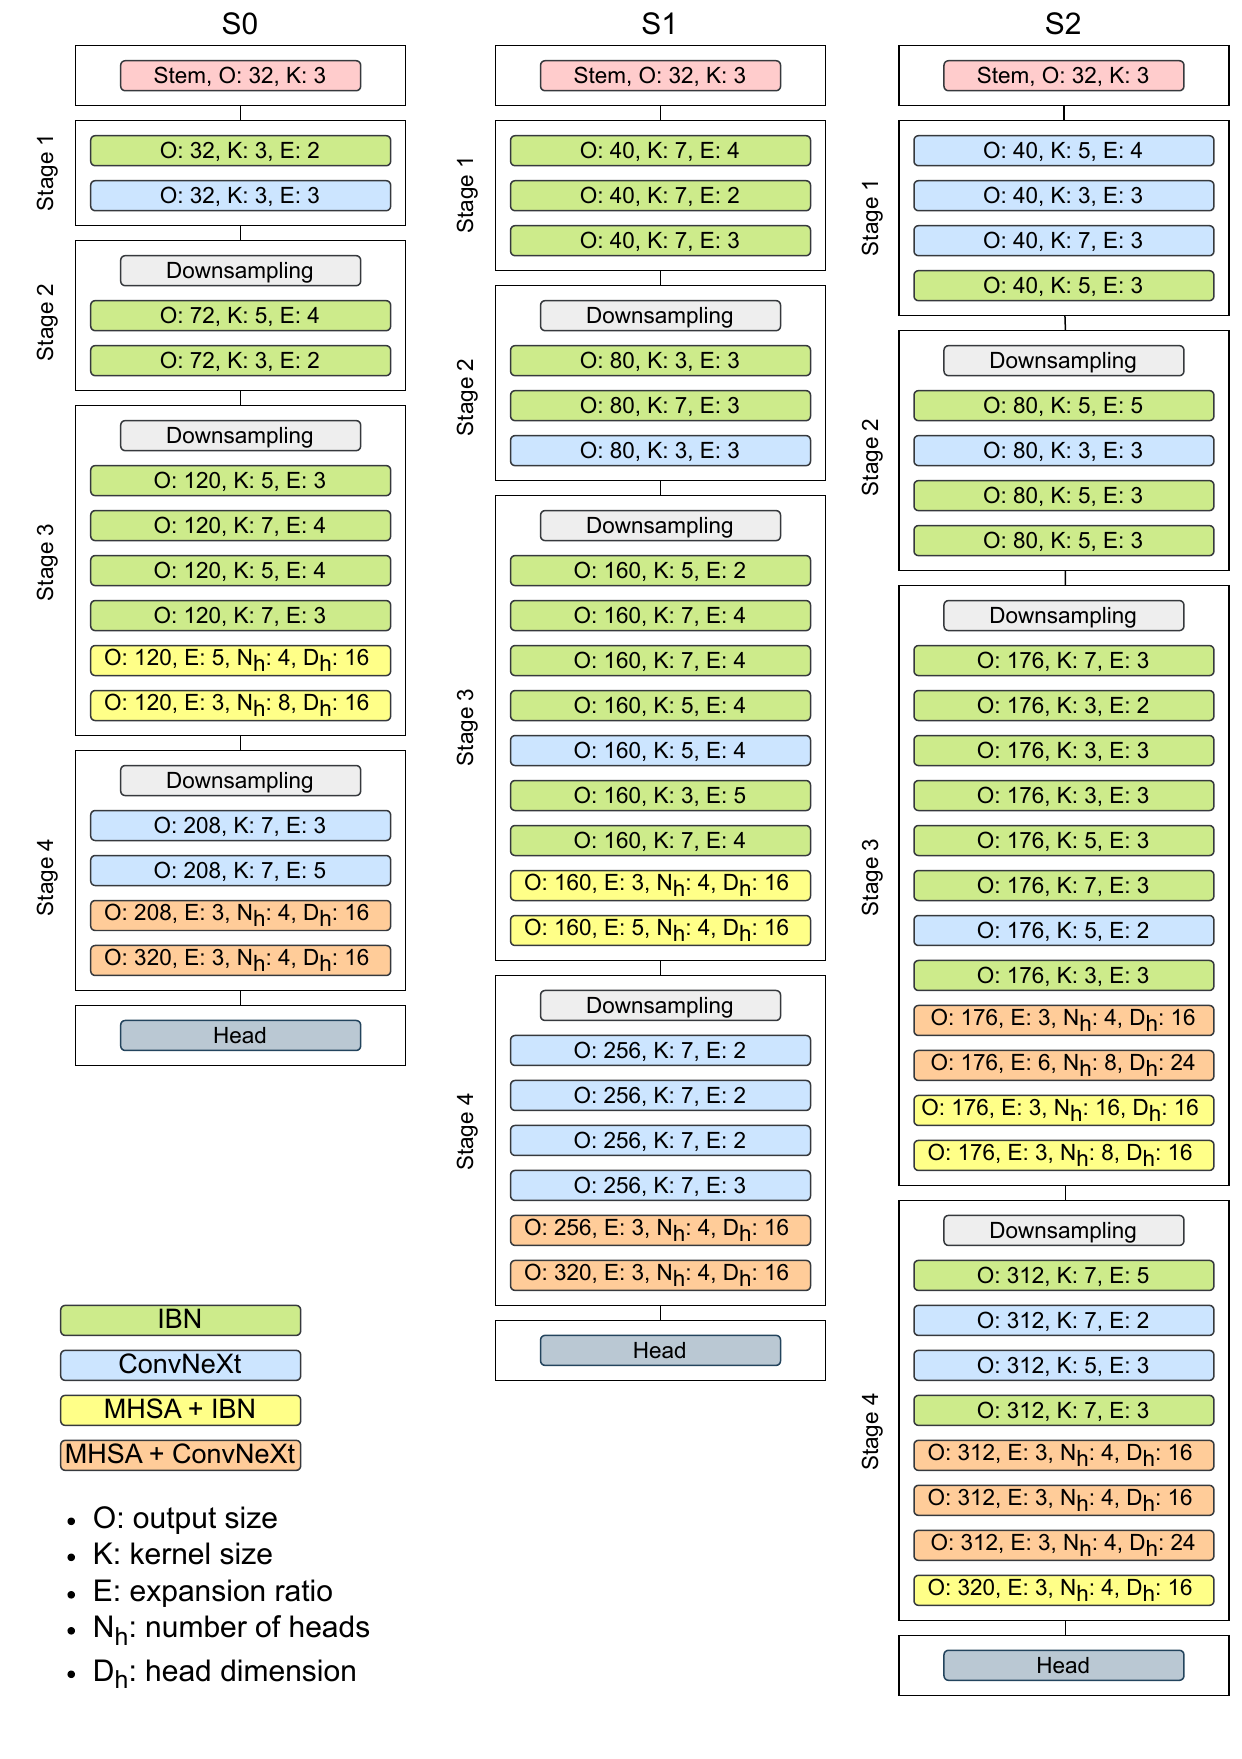}
    \caption{Detailed architectures for ESFormer-S0 (left), S1 (center), S2 (right).}
    \label{fig:nets}
\end{figure*}
%
